# Supplementary material for: The Anisotropy of the Proton Momentum Distribution in Water
Source: arXiv:1805.01193 ancillary file (2018-05-03)
Supplement: Supplementary file 1 [file si.pdf]

# The Anisotropy of the Proton Momentum Distribution in Water

Venkat Kapil,* Alice Cuzzocrea, and Michele Ceriotti

*Laboratory of Computational Science and Modelling, Institute of Materials, Ecole Polytechnique Fédérale de Lausanne, Lausanne, Switzerland*

E-mail: venkat.kapil@epfl.ch

**Abstract**

The document is organized in seven sections. In the first section we outline the well-known derivation of a path integral estimator for the particle momentum distribution using the primitive splitting of the Boltzmann operator. In the second section we derive the particle momentum distribution using an alternate splitting, that is more convenient for implementation in existing PIMD codes. In the third section we derive the scaled gradient estimator. In the fourth section we discuss how to do Molecular dynamics for the ring polymer Hamiltonian obtained by the alternate splitting. In the fifth section we discuss the details of the simulations that were performed. In the sixth section, we present some benchmarks of the accuracy of the neural network potential used to model the short ranged interactions of the MBPOL potential. In the last section we provide the parameters obtained by fitting the proton momentum distributions the various phases of water to a Gauss-Laguerre expansion truncated up to the sixth power.

# Derivation of the particle momentum distribution with the primitive splitting

For the sake of clarity, we consider a one dimensional system described by a Hamiltonian:

$$\hat{H} = \hat{T} + \hat{V} = -\frac{\hbar^2}{2m}\frac{\partial d^2}{\partial dq^2} + V\left(\hat{q}\right) \tag{1}$$

for which an expression for the particle momentum distribution can be written in terms of the off-diagonal elements of the thermal density matrix:

$$\begin{aligned} n(p) &= \left\langle \delta\left(\hat{p} - p\mathbb{1}\right)\right\rangle \\ &= \frac{1}{Z}\int \mathrm{d}q\ \mathrm{d}q'\ \left\langle q\middle|\delta\left(\hat{p} - p\mathbb{1}\right)\middle|q'\right\rangle \left\langle q'\middle|e^{-\beta\hat{H}}\middle|q\right\rangle \\ &= \frac{1}{Z}\int \mathrm{d}q\ \mathrm{d}q'\ (2\pi\hbar)^{-1}e^{i\hbar^{-1}p(q-q')}\left\langle q'\middle|e^{-\beta\hat{H}}\middle|q\right\rangle \\ &= (2\pi\hbar)^{-1}\int \mathrm{d}\mathit{\Delta}\ e^{-i\hbar^{-1}p\mathit{\Delta}}N(\mathit{\Delta}) \end{aligned} \tag{2}$$

with $N(\mathit{\Delta})$, the end-to-end estimator defined as:

$$N(\mathit{\Delta}) = \frac{1}{Z}\int \mathrm{d}q\ \mathrm{d}q'\ \delta(\mathit{\Delta} - q' + q)\left\langle q'\middle|e^{-\beta\hat{H}}\middle|q\right\rangle \tag{3}$$

The familiar path integral expression of the end-to-end estimator can be derived by performing a second order Trotter splitting of the Boltzmann operator:

$$\begin{aligned} N(\mathit{\Delta}) &\approx N_P(\mathit{\Delta}) \\ &= \frac{1}{Z}\int \mathrm{d}q^{(1)}\ \mathrm{d}q^{(P+1)}\ \delta(\mathit{\Delta} - q^{(1)} + q^{(P+1)})\left\langle q^{(1)}\middle|\left[e^{-\beta_P\frac{\hat{V}}{2}}e^{-\beta_P\hat{T}}e^{-\beta_P\frac{\hat{V}}{2}}\right]^P\middle|q^{(P+1)}\right\rangle \\ &= \frac{1}{Z}\int \mathrm{d}\{q^{(j)}\}_{j=1,P+1}\ \delta(\mathit{\Delta} - q^{(1)} + q^{(P+1)})\left[\prod_{j=1}^{P}\left\langle q^{(j)}\middle|\left[e^{-\beta_P\frac{\hat{V}}{2}}e^{-\beta_P\hat{T}}e^{-\beta_P\frac{\hat{V}}{2}}\right]\middle|q^{(j+1)}\right\rangle\right] \end{aligned} \tag{4}$$

with $\beta_P = \beta/P$ and $N(\mathit{\Delta}) = \lim_{P\to\infty} N_P(\mathit{\Delta})$. Upon evaluation of the matrix elements one obtains the following expression for the end-to-end estimator:

$$N_P(\mathit{\Delta}) \propto \int \{\mathrm{d}q^{(j)}\ \}_{j=1,P+1} \delta\left(\mathit{\Delta} - q^{(1)} + q^{(P+1)}\right) e^{-\beta_P \sum_{j=1}^{P}\left[\frac{m\omega_P^2}{2}\left(q^{(j+1)}-q^{(j)}\right)^2+\frac{1}{2}\left(V(q^{(j+1)})+V(q^{(j)})\right)\right]} \tag{5}$$

with $\hbar\omega_P = \beta_P^{-1}$. Upon inclusion of auxiliary momenta, the end-to-end estimator is written, modulo a normalization as the following average:

$$N_P(\mathit{\Delta}) = \left\langle \delta\left(\mathit{\Delta} - q^{(1)} + q^{(P+1)}\right)\right\rangle_{H_P} \tag{6}$$

over the ensemble sampled classically at $\beta_P$ by the isomorphic Hamiltonian:

$$\mathcal{H}_P = \sum_{j=1}^{P+1}\left[\frac{p^{(j)2}}{2m} + \frac{1}{2}m\omega_P^2(q^{(j+1)} - q^{(j)})^2 + \frac{1}{2}\Big(V(q^{(j+1)}) + V(q^{(j)})\Big)\right] \tag{7}$$

# Derivation of the particle momentum distribution with an alternate splitting

A more convenient isomorphic Hamiltonian can be obtained by using the following splitting of the Boltzmann operator:

$$e^{-\beta\hat{\mathcal{H}}} \approx \left[e^{-\beta_P \frac{\hat{T}}{2}} e^{-\beta_P \frac{\hat{V}}{2}}\right]\left[e^{-\beta_P \frac{\hat{V}}{2}} e^{-\beta_P \hat{T}} e^{-\beta_P \frac{\hat{V}}{2}}\right]^{P-1}\left[e^{-\beta_P \frac{\hat{V}}{2}} e^{-\beta_P \frac{\hat{T}}{2}}\right] \tag{8}$$

The path integral expression of the end-to-end estimator can be written as

$$N(\mathit{\Delta}) \approx N_P(\mathit{\Delta}) \tag{9}$$

$$= Z^{-1} \int \{\mathrm{d}q^{(j)}\}_{j=0,P+1} \, \delta(\mathit{\Delta} - q^{(0)} + q^{(P+1)}) \, \left\langle q^{(0)} \middle| \left[ e^{-\beta_P \frac{\hat{V}}{2}} e^{-\beta_P \frac{\hat{T}}{2}} \right] \middle| q^{(1)} \right\rangle \tag{10}$$

$$\times \prod_{j=1}^{P-1} \left[ \left\langle q^{(j)} \middle| \left[ e^{-\beta_P \frac{\hat{V}}{2}} e^{-\beta_P \hat{T}} e^{-\beta_P \frac{\hat{V}}{2}} \right] \middle| q^{(j+1)} \right\rangle \right] \tag{11}$$

$$\times \left\langle q^{(P)} \middle| \left[ e^{-\beta_P \frac{\hat{V}}{2}} e^{-\beta_P \frac{\hat{T}}{2}} \right] \middle| q^{(P+1)} \right\rangle \tag{12}$$

$$= Z^{-1} \int \{\mathrm{d}q^{(j)}\}_{j=0,P} \, \left\langle q^{(0)} \middle| \left[ e^{-\beta_P \frac{\hat{V}}{2}} e^{-\beta_P \frac{\hat{T}}{2}} \right] \middle| q^{(1)} \right\rangle \tag{13}$$

$$\times \prod_{j=1}^{P-1} \left[ \left\langle q^{(j)} \middle| \left[ e^{-\beta_P \frac{\hat{V}}{2}} e^{-\beta_P \hat{T}} e^{-\beta_P \frac{\hat{V}}{2}} \right] \middle| q^{(j+1)} \right\rangle \right] \tag{14}$$

$$\times \left\langle q^{(P)} \middle| \left[ e^{-\beta_P \frac{\hat{V}}{2}} e^{-\beta_P \frac{\hat{T}}{2}} \right] \middle| q^{(0)} - \mathit{\Delta} \right\rangle \tag{15}$$

Upon evaluation of the matrix elements we get

$$N_P(\mathit{\Delta}) \propto \int \{\mathrm{d}q^{(j)}\}_{j=1,P} \left[ \int \mathrm{d}q^{(0)} \, e^{-\frac{m}{\beta_P \hbar^2} \left[ (q^{(1)} - q^{(0)})^2 + (q^{(0)} - \mathit{\Delta} - q^{(P)})^2 \right]} \right] \tag{16}$$

$$\times \, e^{-\beta_P \left[ \sum_{k=1}^{P} V(q^{(j)}) + \sum_{k=1}^{P-1} \frac{m\omega_P^2}{2} (q^{(j+1)} - q^{(j)})^2 \right]} \tag{17}$$

$$= \int \{\mathrm{d}q^{(j)}\}_{j=1,P} \, G\left(\mathit{\Delta}, q^{(1)} - q^{(P)}\right) \, e^{-\beta_P \left[ \sum_{k=1}^{P} V(q^{(j)}) + \sum_{k=1}^{P-1} \frac{m\omega_P^2}{2} (q^{(j+1)} - q^{(j)})^2 \right]} \tag{18}$$

with $G$ defined as:

$$G(x, x') = (2\pi\sigma_P^2)^{-\frac{1}{2}} e^{-\frac{(x-x')^2}{2\sigma_P^2}} \tag{19}$$

Upon inclusion of $P$ auxiliary momenta, the end-to-end estimator is written as the following average:

$$N_P(\mathit{\Delta}) = \left\langle G\left(\mathit{\Delta}, q^{(1)} - q^{(P)}\right)\right\rangle_{H_P} \tag{20}$$

over the ensemble sampled classically by the isomorphic Hamiltonian at $\beta_P$:

$$\mathcal{H}_P = \sum_{j=1}^{P}\left[\frac{{p^{(j)}}^2}{2m} + V(q^{(j+1)})\right] + \sum_{j=1}^{P-1}\left[\frac{1}{2}m\omega_P^2\left(q^{(j+1)} - q^{(j)}\right)^2\right] \tag{21}$$

The derivation can be extended to the case of the case of a many body Hamiltonian in a straightforward manner. The expression for the three dimensional particle momentum distribution comes out to be:

$$n(\mathbf{p}) = (2\pi\hbar)^{-3}\int \mathrm{d}\boldsymbol{\Delta}\ e^{i\hbar^{-1}\mathbf{p}\cdot\boldsymbol{\Delta}}\ N(\boldsymbol{\Delta}) \tag{22}$$

with $N(\boldsymbol{\Delta})$ the end-to-end estimator calculated as the following ensemble average:

$$N(\boldsymbol{\Delta}) \approx N_P(\boldsymbol{\Delta}) = \left\langle G^{3D}\left(\mathit{\Delta}, \boldsymbol{q}_i^{(1)} - \boldsymbol{q}_i^{(P)}\right)\right\rangle_{H_P} \tag{23}$$

where $G^{\mathrm{3D}}$ is a Gaussian Kernel:

$$G^{\mathrm{3D}}(\boldsymbol{x}, \boldsymbol{x}') = (2\pi\sigma_P^2)^{-\frac{3}{2}} e^{-\frac{(\boldsymbol{x}-\boldsymbol{x}')^2}{2\sigma_P^2}} \tag{24}$$

and $H_P$ is a many body ring polymer Hamiltonian defined as:

$$H_P = \sum_{j=1}^{P}\left[\sum_k \frac{[\boldsymbol{p}_k^{(j)}]^2}{2m_k} + \sum_{k\neq i}\frac{1}{2}m_k\omega_P^2[\boldsymbol{q}_k^{(j)} - \boldsymbol{q}_k^{(j+1)}]^2 + V(\boldsymbol{q}^{(j)})\right] + \sum_{j=1}^{P-1}\frac{1}{2}m_i\omega_P^2[\boldsymbol{q}_i^{(j)} - \boldsymbol{q}_i^{(j+1)}]^2 \tag{25}$$

with $\boldsymbol{q}_k^{(j+P)} \equiv \boldsymbol{q}_k^{(j)}$ implied for $j \neq i$.

For isotropic system such a liquids, it is useful to look at the radial momentum distribution which is related to the radial end-to-end estimator by a sine transformation:

$$n(p) = \int \mathrm{d}\mathit{\Delta}\ 4\pi \mathit{\Delta}^2\ N(\mathit{\Delta}) \frac{\sin(p\mathit{\Delta})}{p\mathit{\Delta}} \tag{26}$$

where $N(\mathit{\Delta})$ can be obtained by writing $\boldsymbol{\Delta}$ in spherical coordinates and integrating over polar and azimuthal angles:

$$\begin{aligned} N(\mathit{\Delta}) &\approx N_P(\mathit{\Delta}) \\ &= \int_0^{2\pi} \mathrm{d}\phi \int_{-1}^{1} \mathrm{d}(\cos\theta)\ \left\langle G^{3D}(\boldsymbol{\Delta} - (\mathbf{q}^1 - \mathbf{q}^P)) \right\rangle_{H_P} \\ &= \int_0^{2\pi} \mathrm{d}\phi \int_{-1}^{1} \mathrm{d}(\cos\theta)\ \left\langle (2\pi\sigma_P^2)^{-3/2} e^{\frac{1}{2\sigma_P^2}[-\mathit{\Delta}^2 - (\mathbf{q}^1-\mathbf{q}^P)^2 + 2\mathit{\Delta}|\mathbf{q}^1-\mathbf{q}^P|\cos\theta)]} \right\rangle_{H_P} \\ &= \left\langle \int_0^{2\pi} \mathrm{d}\phi \int_{-1}^{1} \mathrm{d}(\cos\theta)\ (2\pi\sigma_P^2)^{-3/2} e^{\frac{1}{2\sigma_P^2}[-\mathit{\Delta}^2 - (\mathbf{q}^1-\mathbf{q}^P)^2 + 2\mathit{\Delta}|\mathbf{q}^1-\mathbf{q}^P|\cos\theta)]} \right\rangle_{H_P} \\ &= \left\langle G^r(\mathit{\Delta}, \left|\mathbf{q}^1 - \mathbf{q}^P\right|) \right\rangle_{H_P} \end{aligned} \tag{27}$$

that yields the kernel

$$G^r(x, x') = (2\pi\sigma_P^2)^{-1/2} \frac{1}{xx'} \left[ e^{-\frac{1}{2\sigma_P^2}(x-x')^2} - e^{-\frac{1}{2\sigma_P^2}(x+x')^2} \right] \tag{28}$$

# Scaled gradient estimator

We present the derivation of a virial-like estimator for the gradient of the end-to-end estimator which can be defined as:

$$\nabla_{\boldsymbol{\Delta}} N(\boldsymbol{\Delta}) \approx \nabla_{\boldsymbol{\Delta}} N_P(\boldsymbol{\Delta}) = \nabla_{\boldsymbol{\Delta}} \left\langle G^{3D}\left(\boldsymbol{\Delta}, \boldsymbol{q}_i^{(1)} - \boldsymbol{q}_i^{(P)}\right) \right\rangle_{H_P} = \left\langle \nabla_{\boldsymbol{\Delta}} G^{3D}\left(\boldsymbol{\Delta}, \boldsymbol{q}_i^{(1)} - \boldsymbol{q}_i^{(P)}\right) \right\rangle_{H_P} \tag{29}$$

We observing the following properties of the derivative of the 3D Gaussian Kernel:

$$\nabla_{\boldsymbol{\Delta}} G^{3D}\left(\boldsymbol{\Delta}, \boldsymbol{q}_i^{(1)} - \boldsymbol{q}_i^{(P)}\right) = -\nabla_{\boldsymbol{q}_i^{(1)}} G^{3D}\left(\boldsymbol{\Delta}, \boldsymbol{q}_i^{(1)} - \boldsymbol{q}_i^{(P)}\right) = \nabla_{\boldsymbol{q}_i^{(P)}} G^{3D}\left(\boldsymbol{\Delta}, \boldsymbol{q}_i^{(1)} - \boldsymbol{q}_i^{(P)}\right), \tag{30}$$

$$\nabla_{\boldsymbol{q}_i^{(j\neq 1,P)}} G^{3D}\left(\boldsymbol{\Delta}, \boldsymbol{q}_i^{(1)} - \boldsymbol{q}_i^{(P)}\right) = 0 \tag{31}$$

which allow us to write equation (29) in the following form:

$$\nabla_{\boldsymbol{\Delta}} N_P\left(\boldsymbol{\Delta}\right) = \left\langle \sum_{j=1}^{P} \lambda_j \nabla_{\boldsymbol{q}_i^{(j)}} G^{3D}\left(\boldsymbol{\Delta}, \boldsymbol{q}_i^{(1)} - \boldsymbol{q}_i^{(P)}\right)\right\rangle_{H_P} \tag{32}$$

where $\lambda_j$ is an arbitrary sequence with fixed boundary conditions of $\lambda_1 = -\frac{1}{2}$ and $\lambda_P = \frac{1}{2}$. Of the $P$ gradients only those w.r.t the end beads contribute to the average; The rest of them only contribute to the fluctuations of the estimator, which is advantageous since an appropriate choice of $\lambda_k$ should allow us to minimize the variance of the estimator. However, before we proceed to that, we cast equation (32) in a virial like form by integrating by parts:

$$\begin{aligned}
&\nabla_{\boldsymbol{\Delta}} G^{3D}\left(\boldsymbol{\Delta}, \boldsymbol{q}_i^{(1)} - \boldsymbol{q}_i^{(P)}\right) \\
&= \sum_{j=1}^{P} \left\langle \lambda_j \nabla_{\boldsymbol{q}_i^{(j)}} G^{3D}\left(\boldsymbol{\Delta}, \boldsymbol{q}_i^{(1)} - \boldsymbol{q}_i^{(P)}\right)\right\rangle_{H_P} \\
&= \sum_{j=1}^{P} \left\langle \lambda_j G^{3D}\left(\boldsymbol{\Delta}, \boldsymbol{q}_i^{(1)} - \boldsymbol{q}_i^{(P)}\right) \beta_P \nabla_{\boldsymbol{q}_i^{(j)}} H_P\right\rangle_{H_P} \\
&= \left\langle \lambda_j G^{3D}\left(\boldsymbol{\Delta}, \boldsymbol{q}_i^{(1)} - \boldsymbol{q}_i^{(P)}\right) \sum_{j=1}^{P} \left[-\beta_P \boldsymbol{f}_i^{(j)} - \beta_P \boldsymbol{f}_{\mathrm{spr}}^{(j)}\right]\right\rangle_{H_P} \\
&= \left\langle G^{3D}\left(\boldsymbol{\Delta}, \boldsymbol{q}_i^{(1)} - \boldsymbol{q}_i^{(P)}\right) \sum_{j=1}^{P} \left[-\beta_P \lambda_j \boldsymbol{f}_i^{(j)} - \beta_P \lambda_j \boldsymbol{f}_{\mathrm{spr}}^{(j)}\right]\right\rangle_{H_P}
\end{aligned} \tag{33}$$

The spring term can be simplified as follows:

$$-\sum_{j=1}^{P}\beta_P\lambda_j\boldsymbol{f}_{\mathrm{spr}}^{(j)} = m_i\omega_P^2\left[\lambda_1(\boldsymbol{q}_i^{(1)}-\boldsymbol{q}_i^{(2)})+\sum_{j=2}^{P-1}\lambda_j(\boldsymbol{q}_i^{(j)}-\boldsymbol{q}_i^{(j+1)}-\boldsymbol{q}_i^{(j-1)})+\lambda_P(\boldsymbol{q}_i^{(P)}-\boldsymbol{q}_i^{(P-1)})\right] \tag{34}$$

$$= m_i\omega_P^2\left[(\lambda_1-\lambda_2)\boldsymbol{q}_i^{(1)}+\sum_{j=2}^{P-1}[2\lambda_j-\lambda_{j+1}-\lambda_j]\boldsymbol{q}_i^{(j)}+(\lambda_P-\lambda_{P-1})\boldsymbol{q}_i^{(P)}\right] \tag{35}$$

While it would be possible to optimize the $\lambda_k$ based on the computed bead-bead correlations from a reference calculation, we find that results close to the optimum can be obtained taking the $\lambda_k$ is in such a way that the contribution from the spring force coming from intermediate beads vanishes. This condition can be met by imposing that $\lambda_k$ is an arithmetic progression with a common difference of $\frac{1}{P-1}$ for which the fluctuations in the spring term becomes independent of $P$ and the estimator takes the simplified form:

$$\nabla_{\boldsymbol{\Delta}}G^{3D}\left(\boldsymbol{\Delta},\boldsymbol{q}_i^{(1)}-\boldsymbol{q}_i^{(P)}\right) = -\left\langle \boldsymbol{g}\; G^{3D}\left(\boldsymbol{\Delta},\boldsymbol{q}_i^{(1)}-\boldsymbol{q}_i^{(P)}\right)\right\rangle_{H_P} \tag{36}$$

with $\boldsymbol{g}$ the scaled gradient defined as:

$$\boldsymbol{g} = \frac{\sigma_P^{-2}}{1-P^{-1}}\left[(\boldsymbol{q}_i^{(1)}-\boldsymbol{q}_i^{(P)})\right]+\sum_{j=1}^{P}\beta_P\lambda_j\boldsymbol{f}_i^{(j)} \tag{37}$$

We also derive the derivative of the radial end-to-end estimator by simply integrating the Gaussian kernel over azimuthal and polar angles:

$$N'(\mathit{\Delta}) \approx N'_P(\mathit{\Delta}) \tag{38}$$

$$= \int_0^{2\pi} \mathrm{d}\phi \int_{-1}^{1} \mathrm{d}(\cos\theta)\ \frac{\partial}{\partial \mathit{\Delta}}\ \left\langle G^{3D}(\mathbf{\Delta} - (\mathbf{q}^1 - \mathbf{q}^P)) \right\rangle_{H_P} \tag{39}$$

$$= \int_0^{2\pi} \mathrm{d}\phi \int_{-1}^{1} \mathrm{d}(\cos\theta)\ \frac{\partial}{\partial \mathit{\Delta}}\ \left\langle G^{3D}(\mathit{\Delta}, \left|\mathbf{q}_i^1 - \mathbf{q}_i^P\right|, \theta) \right\rangle_{H_P} \tag{40}$$

$$= \int_0^{2\pi} \mathrm{d}\phi \int_{-1}^{1} \mathrm{d}(\cos\theta)\ \left[\frac{\partial \mathit{\Delta}_x}{\partial \mathit{\Delta}} \frac{\partial}{\partial \mathit{\Delta}_x} + \frac{\partial \mathit{\Delta}_y}{\partial \mathit{\Delta}} \frac{\partial}{\partial \mathit{\Delta}_y} + \frac{\partial \mathit{\Delta}_z}{\partial \mathit{\Delta}} \frac{\partial}{\partial \mathit{\Delta}_z}\right]\ \left\langle G^{3D}(\mathit{\Delta}, \left|\mathbf{q}_i^1 - \mathbf{q}_i^P\right|, \theta) \right\rangle_{H_P} \tag{41}$$

$$= \int_0^{2\pi} \mathrm{d}\phi \int_{-1}^{1} \mathrm{d}(\cos\theta)\ \left\langle \left[g_x \sin\theta\cos\phi + g_y \sin\theta \sin\phi + g_z \cos\theta\right]\ G^{3D}(\mathit{\Delta}, \left|\mathbf{q}_i^1 - \mathbf{q}_i^P\right|, \theta) \right\rangle_{H_P} \tag{42}$$

$$= 2\pi \int_{-1}^{1} \mathrm{d}(\cos\theta)\ \left\langle [g_z \cos\theta]\ G^{3D}(\mathit{\Delta}, \left|\mathbf{q}_i^1 - \mathbf{q}_i^P\right|, \theta) \right\rangle_{H_P} \tag{43}$$

$$= \left\langle \left[\boldsymbol{g} \cdot \frac{\mathbf{q}_i^{(1)} - \mathbf{q}_i^{(P)}}{\left|\mathbf{q}_i^{(1)} - \mathbf{q}_i^{(P)}\right|} \frac{\mathbf{q}_i^{(1)} - \mathbf{q}_i^{(P)}}{\left|\mathbf{q}_i^{(1)} - \mathbf{q}_i^{(P)}\right|}\right]\ G^{\mathrm{dr}}(\mathit{\Delta}, \delta) \right\rangle_{H_P} \tag{44}$$

with the kernel defined as:

$$G^{\mathrm{dr}}(x, x') = (2\pi\sigma_P^2)^{-1/2} \left(x'x\right)^{-2} \left[e^{-\frac{(x'+x)^2}{2\sigma_P^2}} \left(xx' + \sigma_P^2\right) + e^{-\frac{m_i\left(x'-x\right)^2}{2\sigma_P^2}} \left(xx' - \sigma_P^2\right)\right] \tag{45}$$

# Molecular Dynamics and Ring Polymer Contraction

The ring polymer Hamiltonian can be rewritten as:

$$H_P = H_P^{\mathrm{c}} + H_P^{\mathrm{o}} + \sum_{j=1}^{P} V(\boldsymbol{q}^{(j)}) \tag{46}$$

where

$$H_P^{\mathrm{c}} = \sum_{j=1}^{P} \left[ \sum_{k \neq i} \frac{[\boldsymbol{p}_k^{(j)}]^2}{2m_k} + \sum_{k \neq i} \frac{1}{2} m_k \omega_P^2 [\boldsymbol{q}_k^{(j)} - \boldsymbol{q}_k^{(j+1)}]^2 \right] \tag{47}$$

and

$$H_P^{\mathrm{c}} = \sum_{j=1}^{P} \left[ \frac{[\boldsymbol{p}_i^{(j)}]^2}{2m_k} + \frac{1}{2} m_k \omega_P^2 [\boldsymbol{q}_i^{(j)} - \boldsymbol{q}_i^{(j+1)}]^2 \right] \tag{48}$$

Normal Mode PIMD can be performed by altering the scheme used by Ceriotti and co-workers in i-PI[1] by applying a Trotter splitting on the Louiville propagator of $H_P$:

$$e^{iL_P \delta t} = e^{i[L_V + L_{\mathrm{c}} + L_{\mathrm{o}}]\delta t} \approx e^{iL_V \delta t/2} e^{iL_{\mathrm{c}} \delta t} e^{iL_{\mathrm{o}} \delta t} e^{iL_V \delta t/2} \tag{49}$$

The algorithm can be written as

$$p_k^{(j)} \to p_k^{(j)} + \frac{\partial V(\{\boldsymbol{q}\})}{\partial q_k^{(j)}}\delta t/2 \tag{50}$$

$$\tilde{p}_{k\neq i}^{(j)} \to \sum_{l=1}^{P} p_{k\neq i}^{(l)} c_{lj}^{(c)} \quad \tilde{q}_{k\neq i}^{(j)} \to \sum_{l=1}^{P} q_{k\neq i}^{(l)} c_{lj}^{(c)} \tag{51}$$

$$\begin{bmatrix} \tilde{p}_{k\neq i}^{(j)} \\ \tilde{q}_{k\neq i}^{(j)} \end{bmatrix} \to \begin{bmatrix} \cos \Omega_j^{(\mathrm{c})}\delta t & -m_{k\neq i}\Omega_j^{(\mathrm{c})} \sin \Omega_j^{(\mathrm{c})}\delta t \\ \left(m_{k\neq i}\Omega_j^{(\mathrm{c})}\right)^{-1} \sin \Omega_j^{(\mathrm{c})}\delta t & \cos \Omega_j^{(\mathrm{c})}\delta t \end{bmatrix} \begin{bmatrix} \tilde{p}_{k\neq i}^{(j)} \\ \tilde{q}_{k\neq i}^{(j)} \end{bmatrix} \tag{52}$$

$$p_i^{(j)} \to \sum_{l=1}^{P} \tilde{p}_i^{(l)} c_{lj}^{(c)} \quad q_i^{(j)} \to \sum_{l=1}^{P} \tilde{q}_i^{(l)} c_{lj}^{(c)} \tag{53}$$

$$\tilde{p}_i^{(j)} \to \sum_{l=1}^{P} p_i^{(l)} c_{lj}^{(o)} \quad \tilde{q}_i^{(j)} \to \sum_{l=1}^{P} q_i^{(l)} c_{lj}^{(o)} \tag{54}$$

$$\begin{bmatrix} \tilde{p}_i^{(j)} \\ \tilde{q}_i^{(j)} \end{bmatrix} \to \begin{bmatrix} \cos \Omega_j^{(\mathrm{o})}\delta t & -m_i\Omega_j^{(\mathrm{o})} \sin \Omega_j^{(\mathrm{o})}\delta t \\ \left(m_i\Omega_j^{(\mathrm{o})}\right)^{-1} \sin \Omega_j^{(\mathrm{o})}\delta t & \cos \Omega_j^{(\mathrm{o})}\delta t \end{bmatrix} \begin{bmatrix} \tilde{p}_i^{(j)} \\ \tilde{q}_i^{(j)} \end{bmatrix} \tag{55}$$

$$p_i^{(j)} \to \sum_{l=1}^{P} \tilde{p}_i^{(l)} c_{lj}^{(o)} \quad q_i^{(j)} \to \sum_{l=1}^{P} \tilde{q}_i^{(l)} c_{lj}^{(o)} \tag{56}$$

$$p_k^{(j)} \to p_k^{(j)} + \frac{\partial V(\{\boldsymbol{q}\})}{\partial q_k^{(j)}}\delta t/2 \tag{57}$$

where $\{\Omega_j^{(c)},\, c_{lj}^{(c)}\}$ and $\{\Omega_j^{(o)},\, c_{lj}^{(o)}\}$ correspond to the set of eigenvalues and eigenvectors of the dynamical matrices of the closed and open polymer of a free particle respectively. If range separation is possible, one can use a Multiple Time Step Algorithm, as well as an open-path version of Ring Polymer Contraction,[2] adapting the implementation of Ref. 3 by simply replacing the eigenvectors of the free ring polymer by those of an open polymer.

# Simulation protocol

Both open and closed PIMD simulations were performed using i-PI, a Python wrapper for (path integrals) molecular dynamics.[1] S ince proton momentum distribution and quantum kinetic energy are dominated by short range interactions, we were able to use small simulations

cells of water and ice containing 64 molecules and 96 molecules respectively at experimental densities. For simulating ice 4 proton disordered structures were used. Energies and forces were computed using as driver codes DLPOLY[4] for MBPOL, LAMMPS[5] for q-TIP4P/f, and an implementation of the neural network potential in LAMMPS[6] for NN-B3LYP+D3.

In order to the calculate kinetic energies listed in table 1 of the manuscript, $NVT$ closed path PIMD simulations were performed using 64 beads. A centroid-virial estimator[7] was used to evaluate the kinetic energy. For B3LYP+D3 and q-TIP4P/f water a timestep of 0.25 fs was used while for MBPOL an implementation[3] of multiple time step algorithm[8] was used. A NN potential that describes the short range interactions effectively, fitted to MBPOL reference calculations using RuNNer,[9] was integrated in the inner most loop with a timestep of 0.25 fs and the difference between the MBPOL and NN was integrated with an outer timestep of 1.00 fs. While the NN was evaluated on a ring polymer of 64 beads the difference potential was evaluated on contracted replica of 8 beads and extrapolated using a Ring Polymer Contraction scheme.[2] A PILE-G[10] thermostat with a time constant of 10 fs was used to enforce canonical sampling.

The open PIMD simulations were performed with one open path per molecule with the same setup as described in the previous paragraph. The end-to-end vector and the forces acting on the target atoms were printed out every 2 fs. The momentum distributions were calculated using the scaled gradient estimator from 40 ps long simulations. For ice, distributions obtained from different starting configurations were further averaged. Longer benchmark calculations with a single open path per simulation were also performed, and used to generate Fig. 1 in the main text.

The $NPT$ open and closed path simulations were performed using the Bussi-Zykova-Parrinello barostat modified for constant pressure PIMD[1] with 64 beads. In case of open PIMD one path per molecule was opened. The time constant of the barostat was set to 200 fs. A Langevin thermostat of time constant 100 fs and PILE-G thermostat with a time

constant of 10 fs were used applied to the barostat and the ring polymer degrees of freedom. In order to speed up the simulations of q-TIP4P/f and B3LYP+D3 water we used a *BAOAB* integrator[11] with a timestep of 0.5 fs which gives results that are indistinguishable from those obtained from a standard integrator with a time step of 0.25 fs. For MBPOL water the MTS protocol discussed in the previous paragraph was used. The scaled gradient estimator was used to calculate the proton momentum distributions from 20-ps long simulations.

## Accuracy of the MTS scheme

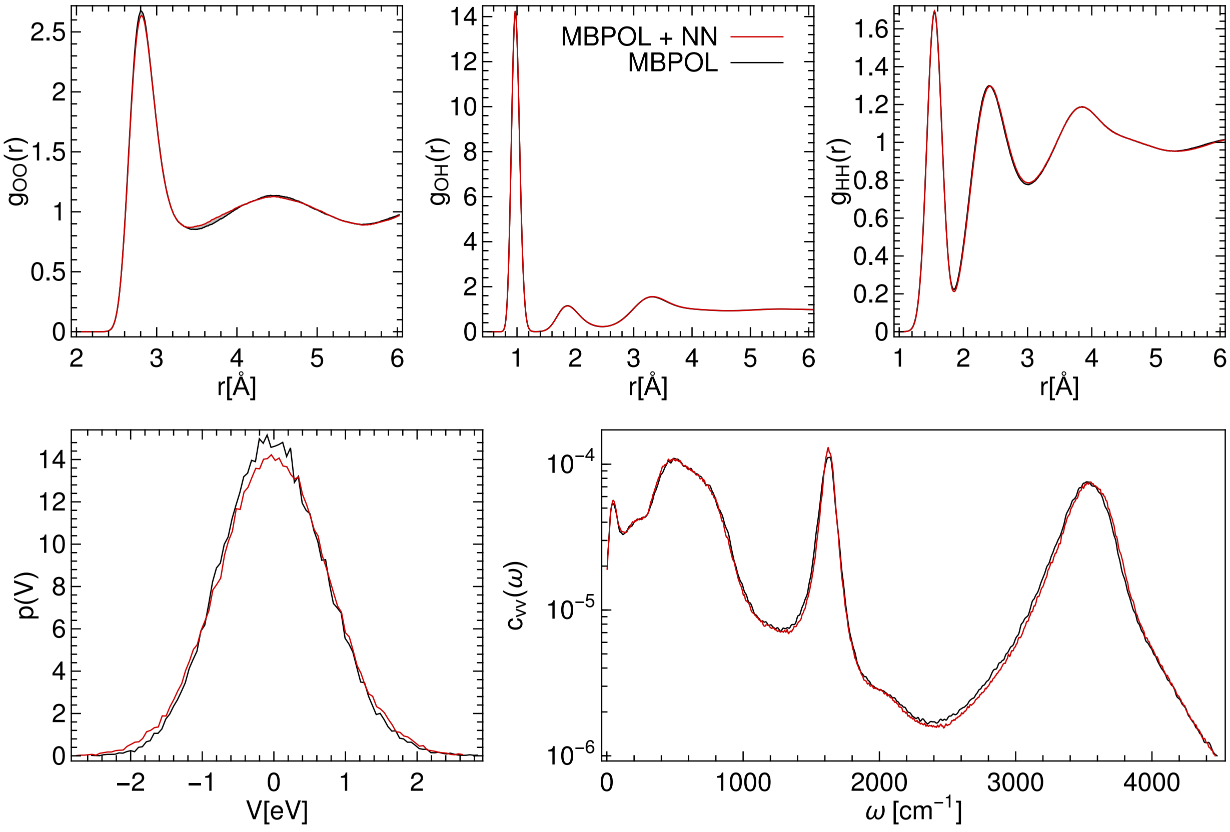


Figure S1: The top panels show the OO (left), OH (middle) and HH (right) pair correlation functions calculated from a 100 ps long PIMD simulation using the MBPOL potential (black) and the MTS simulation using the NN and the MBPOL simulation (black) of the same length. The lower panels show the fluctuation of the potential energy about its average (left) and the vibrational density of states.

Following the protocol of Imbalzano and co-workers[12] to select an appropriate set of

symmetry functions, a high dimensional neural network (NN) framework, introduced by Behler and Parrinello,[13] was used to fit[9] a short ranged NN to reproduce the energetics of MBPOL water. Figure S1 shows a few observables computed from a reference *NVT* PIMD simulation of 64 molecules water at 300 K compared with those obtained from one that uses the MTS scheme[3] with the NN potential as a short ranged component and the difference between MBPOL and the NN as the long ranged component. A time step of 0.25 fs and 32 beads were used for the reference simulation. For the MTS simulation, the NN was computed on 32 beads and integrated with a timestep of 0.25 fs while the difference potential was computed every 1 fs on 4 beads. The upper panels show the pair correlation functions while the lower ones show that fluctuation of the potential and the vibrational density of states (VDOS). The overall agreement with the reference is excellent with minute differences that are within the statistical error bars of the calculations.

## Fitting the momentum distribution to the Gauss-Laguerre expansion

As a reference for future DINS studies we also fit the proton momentum distributions obtained from simulations to a Gauss-Laguerre expansion:

$$4\pi p^2 n_{\mathrm{M}}(p) = \left(\sqrt{2\pi}\sigma\right)^{-3} 4\pi p^2 e^{-\frac{1}{2}p^2\sigma^{-2}} \left[1 + \sum_{k=2}^{\infty} c_k (-1)^k L_k^{\frac{1}{2}}\left(\frac{1}{2}p^2\sigma^{-2}\right)\right] \tag{58}$$

where, $L_k^{\frac{1}{2}}(x)$ is the Generalized Laguerre Polynomial in $x$. The model sheds light on how much the distribution deviates from an effective Maxwell-Boltzmann distribution. The fit was performed using the software MATHEMATICA 10.0 with the series truncated up to the sixth power. The values of the coefficients are listed in table S1.

Table S1: The $c_2$, $c_4$, $c_6$ coefficients and the width $\sigma$ obtained by fitting the radial proton momentum distribution to equation 58 for various phases of B3LYP+D3, MBPOL and q-TIP4P/f water.

| Phase | B3LYP+D3 $(c_2, c_4, c_6, \sigma[\text{Å}^{-1}])$ | MBPOL $(c_2, c_4, c_6, \sigma[\text{Å}^{-1}])$ | q-TIP4P/f $(c_2, c_4, c_6, \sigma[\text{Å}^{-1}])$ |
|---|---|---|---|
| 271 K [SW] | (0.174, 0.020, 0.015, 4.967) | (0.187, 0.024, 0.020, 4.997) | (0.182, 0.022, 0.019, 4.997) |
| 271 K [$I_h$] | (0.147, 0.011, 0.010, 4.966) | (0.179, 0.021, 0.017, 5.017) | (0.165, 0.019, 0.014, 5.020) |
| 300 K [W] | (0.166, 0.024, 0.014, 4.952) | (0.195, 0.026, 0.021, 5.027) | (0.181, 0.024, 0.018, 5.026) |

# References


(1) Ceriotti, M.; More, J.; Manolopoulos, D. E. i-PI: A Python interface for ab initio path integral molecular dynamics simulations. *Comp. Phys. Comm.* **2014**, *185*, 1019–1026.

(2) Markland, T. E.; Manolopoulos, D. E. An efficient ring polymer contraction scheme for imaginary time path integral simulations. *J. Chem. Phys.* **2008**, *129*, 024105.

(3) Kapil, V.; VandeVondele, J.; Ceriotti, M. Accurate molecular dynamics and nuclear quantum effects at low cost by multiple steps in real and imaginary time: Using density functional theory to accelerate wavefunction methods. *J. Chem. Phys.* **2016**, *144*, 054111.

(4) Smith, W.; Forester, T. DL_POLY_2.0: A general-purpose parallel molecular dynamics simulation package. *Journal of Molecular Graphics* **1996**, *14*, 136 – 141.

(5) Plimpton, S. Fast Parallel Algorithms for Short-Range Molecular Dynamics. *J. Comp. Phys.* **1995**, *117*, 1–19.

(6) Singraber, A.; Morawietz, T.; Behler, J.; Dellago, C. *to be published*

(7) Kolár, M.; O'Shea, S. F. A high-temperature approximation for the path-integral quantum Monte Carlo method. *Journal of Physics A: Mathematical and General* **1996**, *29*, 3471.

(8) Tuckerman, M.; Berne, B. J.; Martyna, G. J. Reversible multiple time scale molecular dynamics. *J. Chem. Phys.* **1992**, *97*, 1990.

(9) RuNNer - A Neural Network Code for High-Dimensional Potential-Energy Surfaces, Jörg Behler, Lehrstuhl für Theoretische Chemie, Ruhr-Universität Bochum, Germany.

(10) Ceriotti, M.; Parrinello, M.; Markland, T. E.; Manolopoulos, D. E. Efficient stochastic thermostatting of path integral molecular dynamics. *J. Chem. Phys.* **2010**, *133*, 124104.

(11) Leimkuhler, B.; Matthews, C. Robust and efficient configurational molecular sampling via Langevin dynamics. *The Journal of Chemical Physics* **2013**, *138*, 174102.

(12) Imbalzano, G.; Anelli, A.; Giofré, D.; Klees, S.; Behler, J.; Ceriotti, M. Automatic selection of atomic fingerprints and reference configurations for machine-learning potentials. *The Journal of Chemical Physics* **2018**, *148*, 241730.

(13) Behler, J.; Parrinello, M. Generalized Neural-Network Representation of High-Dimensional Potential-Energy Surfaces. *Phys. Rev. Lett.* **2007**, *98*, 146401.
